# Supplementary material for: Prioritized training on points that are learnable, worth learning, and not yet learned (workshop version)
Source: arXiv:2107.02565 source file (2023-10-17)
Supplement: Supplementary file 1 [file appendix.tex]

\section{Appendix}
